# Supplementary material for: Screenplay Quality Assessment: Can We Predict Who Gets Nominated?
Source: arXiv:2005.06123 source file (2020-05-13)
Supplement: Supplementary file 1 [file appendix.tex]

\section{Features}
\label{sec:features}

\textit{Characterization} and \textit{Plot} are two main aspects of focus in the industry. We review narratology literature and bases on which we compute six features. For each aspect, we provide some intuitive motivations, and then detail how we convert them computationally. 

According to \citet{weiland2018structure}, who proposed a general guideline as to where important events should be positioned, a script should place nine SPs roughly equally distributed, creating eight almost equal-lengthed segments in between. \ming{do we need a table for this? like (SP, \%) pairs} We hypothesize that such structural hints should help to achieve our objective. Based on the statistics of both dataset, to leverage the SPs, we collect a context window of 270 words centered at SPs for all scripts. \ming{I kinda want to put this paragraph in the Narratology Model section, and move the Featrue section after Narratology Model, so the sections look mor balanced.}

\subsection{Characterization}

By the definition of characterization, we hypothesize that by measuring pattern change of characters, we may see how writers develop the characters' personality. We seek pattern change via two kinds of changes writers would make between SPs - linguistic (speaking pattern) change and emotional change. For linguistic change, we extract the dependency trees of the character; for emotional change we use normalized Empath \citep{Fast2016EmpathUT} to score characters' emotion status. 
Besides, as \citet{kao-jurafsky-2012-computational} show, in poetry, the type-token ratio most positively relate to the quality of a poem. We believe that this concept should work similarly on character analysis, and can show how much effort writers put in in characterization. 

For \textit{characterization}, we choose the top two most speaking characters of each movie to analyze.

\smallskip\noindent
\textbf{Linguistic Activity Curve.}   
We apply \textit{activity curve} \cite{dawadi2016modeling} to model lexical linguistic curve based on the lexical distribution of the speaking utterances, it uese a Permutation-based Change Detection in Activity Routine (PCAR) algorithm to calculate the change between two windows of lexical distributions.

\smallskip\noindent
\textbf{Emotional Activity Curve.} Similar to the previous one, once we get normalized Empath score, we follow the same PCAR to compute this feature.

\smallskip\noindent
\textbf{Type-token ratio.} We compute this by computing the number of unique words used by a character and then divided by the total number of words. 

\subsection{Plot}

We hypothesize that a well-written dramatic event should have certain emotional effect to readers and thus writers may use stronger words to achieve that. Therefore, we examine this hypothesis by leveraging two sentiment analysis lexicons to compute the emotional strength of SPs.

Also, since events are usually adressed in units of  scenes, we apply simple clustering techniques on autoencoder results on pycholinguistic  (provided by Empath) features at the scence level, to a picture of how many different emotionally similar scenes across the dataset appear in a movie.

\smallskip\noindent
\textbf{Valence-Arousal-Dominance (VAD).} \citet{vad-acl2018} performed extensive study in getting an objective score for words in VAD dimensional space \citep{Russell1980ACM, Russell2003CoreAA}. We compute average scores over the context window of each SP.

\smallskip\noindent
\textbf{Emotion Intensity.} Similar to VAD, we use the NRC Affect Intensity Lexicon \citep{LREC18-AIL} over the SPs to score emotion intensity along four basic emotion classes \citep{PLUTCHIK19803}.

\smallskip\noindent
\textbf{Empath Clustering.} We use Empath \citep{Fast2016EmpathUT} to extract lexical categories for each uttrance. We then cluter the lexical category distributions of utterances using deep embedded clustering \cite{xie2016unsupervised}. We compute the cluster distribution given all utterances within a movie as the feature representation of a movie.

\subsection{Analysis}
We visualize partial features from ScriptBase in a ``nomination v non-nomination" fashion to show the potential of our features. For some we can easily observe clear differences from one to the other, while some are more subtle. For instance, Speaking pattern of Role 2 is ambiguous between the two classes, as shown in Fig.~\ref{fig:linguistic}, and yet we can easily discern nominated scripts by Arousal as in Fig.~\ref{fig:arousal}.

\ming{Need to reorganize the plots. But may have to choose only a couple to show?}

\begin{figure}[h]
    \centering
    \includegraphics[width=0.5\textwidth]{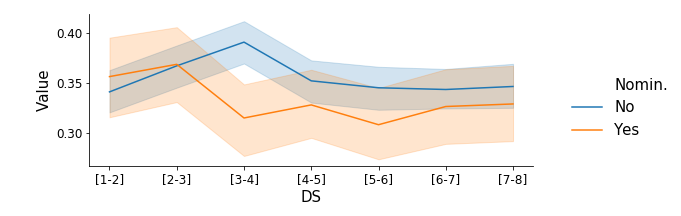}
    \caption{Role2 of Linguistic Activity Curve of ScriptBase}
    \label{fig:linguistic}
\end{figure}

\begin{figure}[h]
    \centering
    \includegraphics[width=0.5\textwidth]{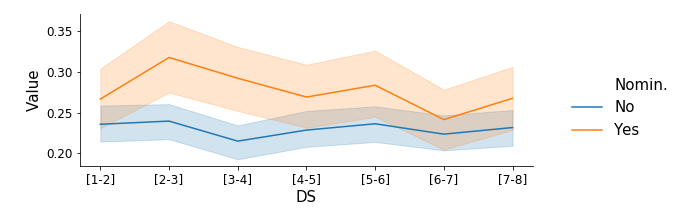}
    \caption{Role1 of Emotional Activity Curve of ScriptBase}
    \label{fig:mesh1}
\end{figure}
\begin{figure}[h]
    \centering
    \includegraphics[width=0.5\textwidth]{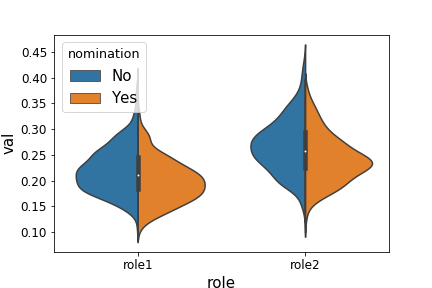}
    \caption{Type-token of ScriptBase}
    \label{fig:mesh1}
\end{figure}
\begin{figure}[h]
    \centering
    \includegraphics[width=0.5\textwidth]{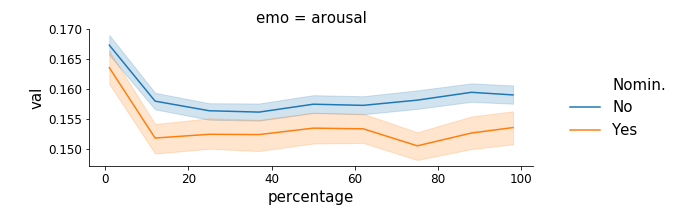}
    \caption{Arousal in VAD of ScriptBase}
    \label{fig:arousal}
\end{figure}
\begin{figure}[h]
    \centering
    \includegraphics[width=0.5\textwidth]{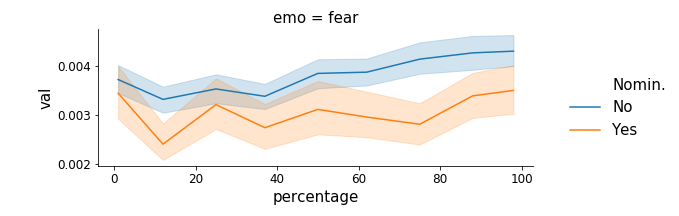}
    \caption{Fear in Emotion Intensity of ScriptBase}
    \label{fig:mesh1}
\end{figure}
\begin{figure}[h]
    \centering
    \includegraphics[width=0.5\textwidth]{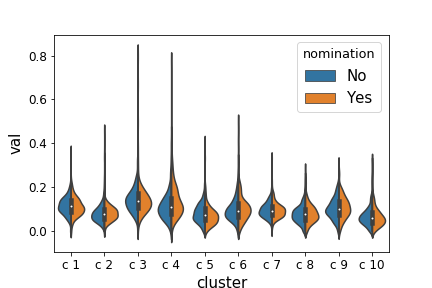}
    \caption{Empath Clustering of ScriptBase}
    \label{fig:mesh1}
\end{figure}

\begin{figure}[h]
    \centering
    \includegraphics[width=0.5\textwidth]{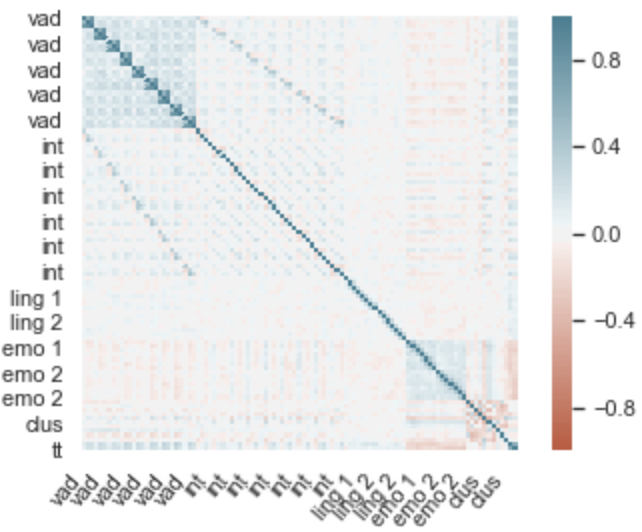}
    \caption{Feature correlation of ScriptBase}
    \label{fig:mesh1}
\end{figure}
